# Supplementary material for: Predicting the Generalization Gap in Deep Networks with Margin Distributions
Source: arXiv:1810.00113 source file (2019-06-12)
Supplement: Supplementary file 1 [file appendix3.tex]

\newpage
\section{Appendix: Unnormalized and Normalized Distributions}
\label{sec:compare_dists}
